# Supplementary material for: VisuLogic: A Benchmark for Evaluating Visual Reasoning in Multi-modal Large Language Models
Source: arXiv:2504.15279 source file (2025-04-21)
Supplement: Supplementary file 1 [file caption_benchmark.tex]

\section{Caption Examples}
% 我们在实验中使用了LLM作为对比实验。我们使用GPT-4o来获得图像的caption, 
In our experiment, we used an LLM as a comparative experiment. When setting up the LLM experiment, we first used GPT-4o to convert images into captions. As shown in the Figure~\ref{fig:benchmark_des_len_comparison}, we used the tokenizers of two commonly used open-source models to analyze the token length of the caption benchmark. We provide more examples of image captions shown in Figure~\ref{fig:image_cation1} and Figure~\ref{fig:image_cation2}.
\begin{figure}
    \centering
    \includegraphics[width=1\linewidth]{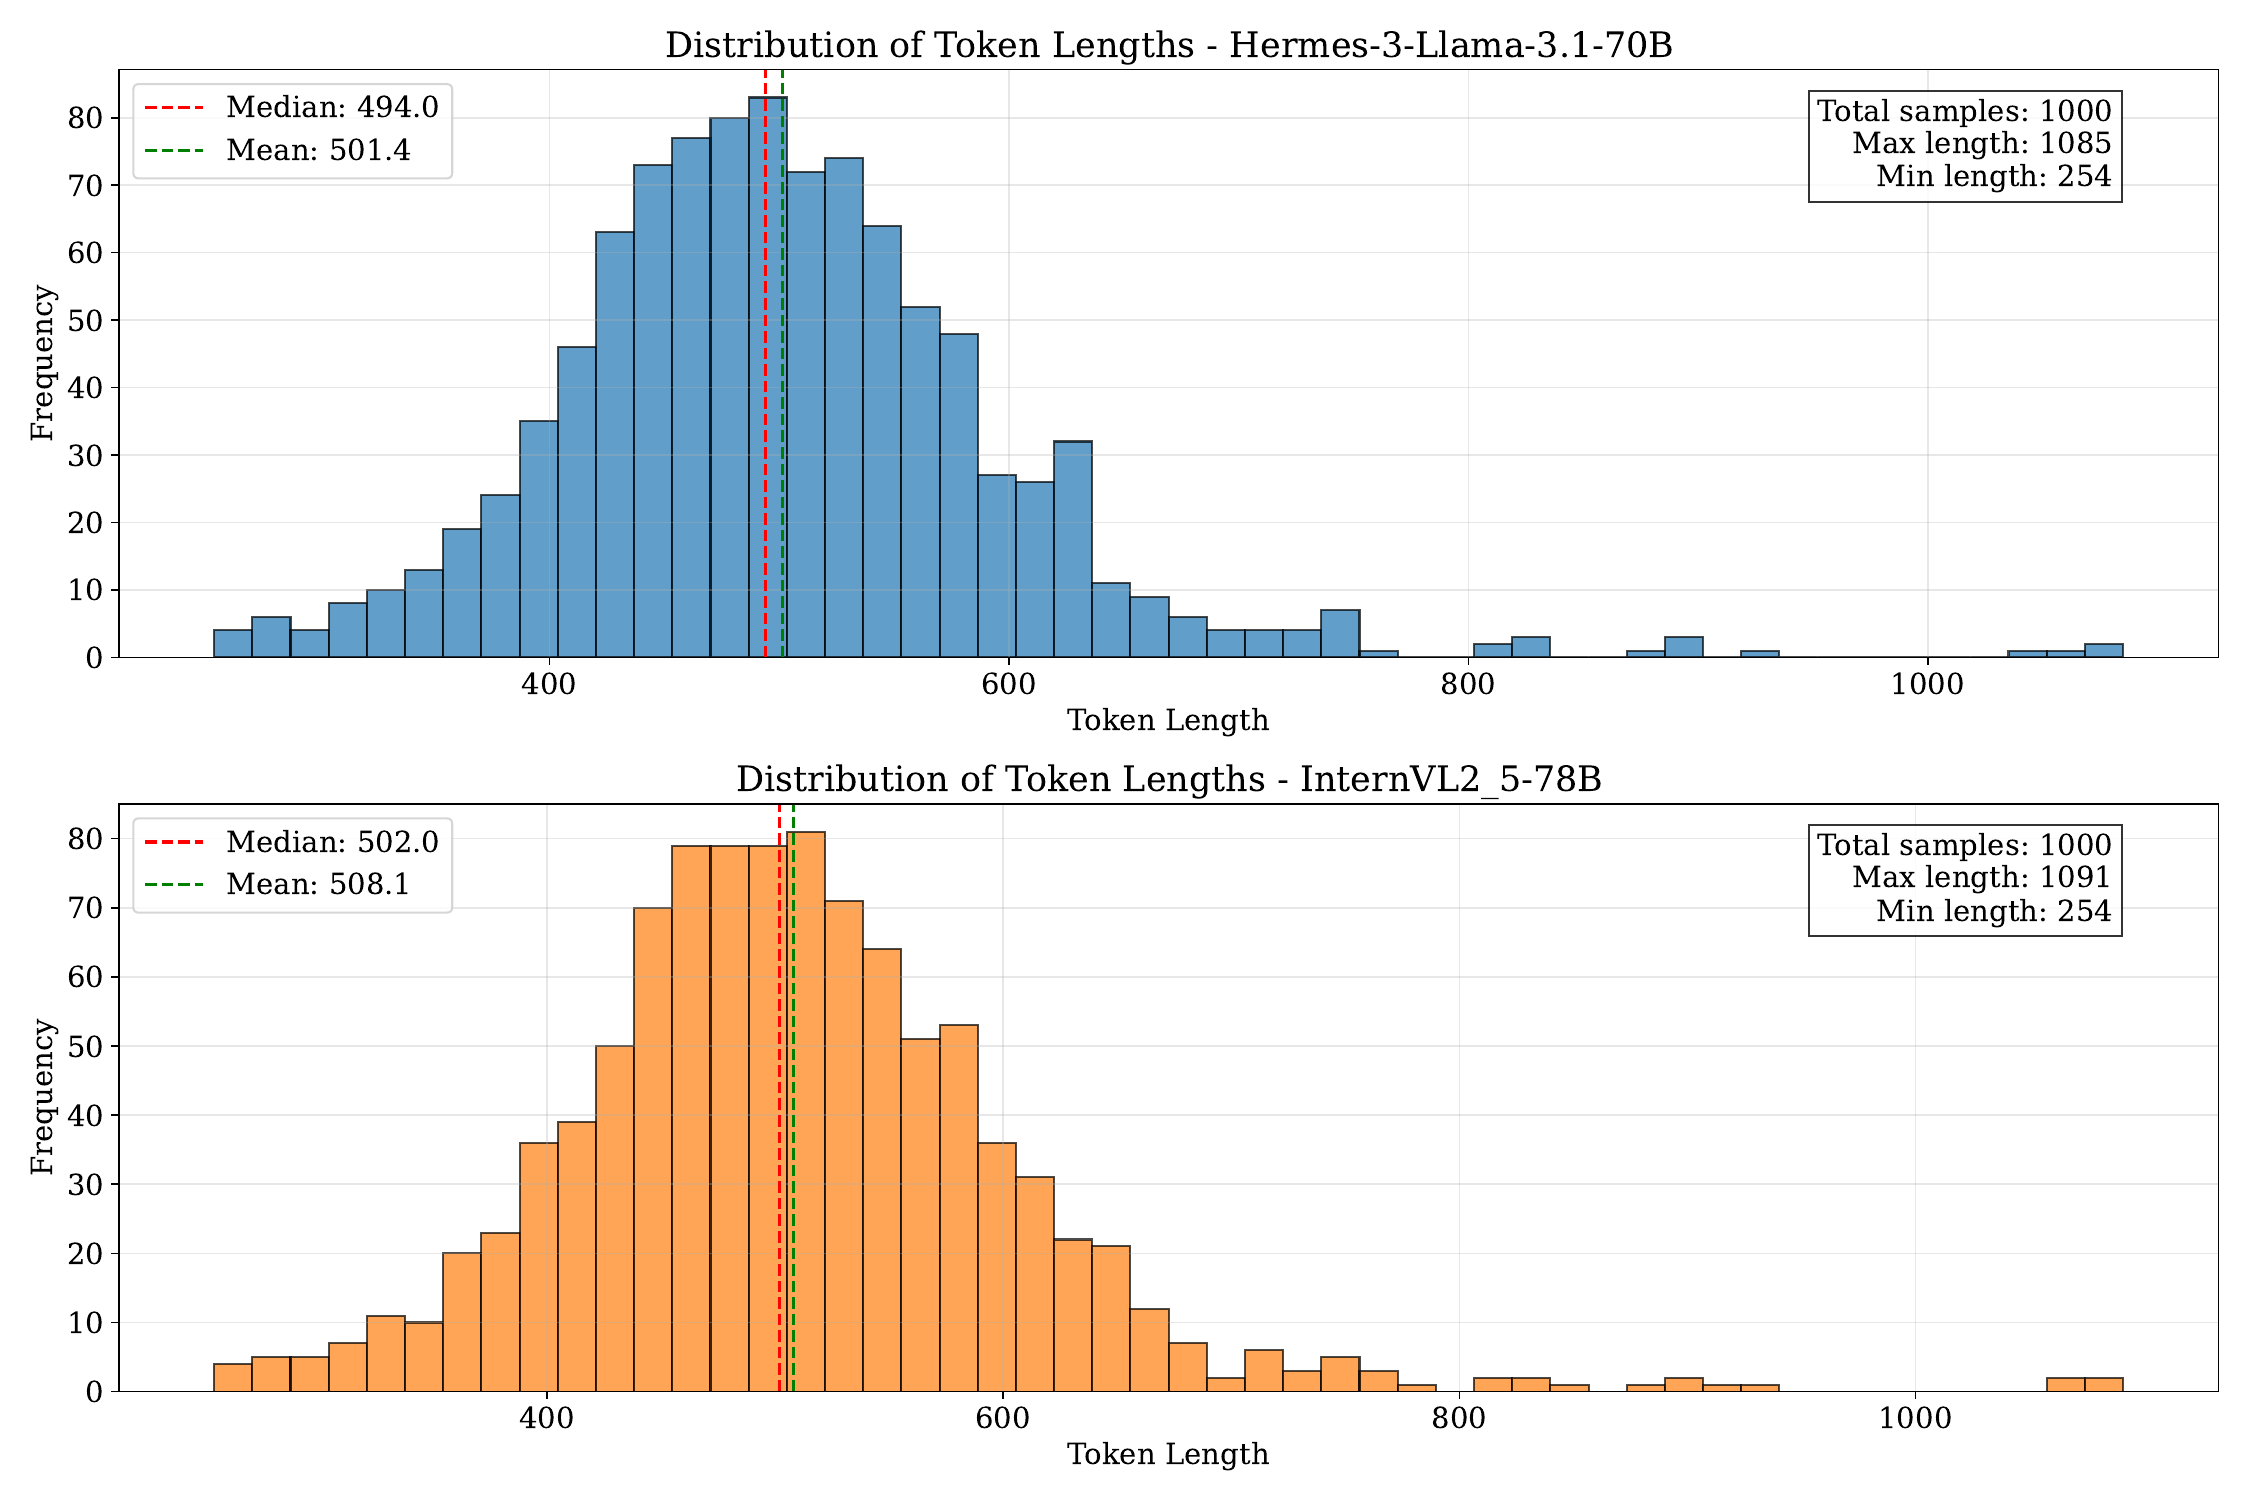}
    \caption{Distribution of benchmark with image caption.}
    \label{fig:benchmark_des_len_comparison}
\end{figure}

\begin{figure}
    \centering
    \includegraphics[width=1\linewidth]{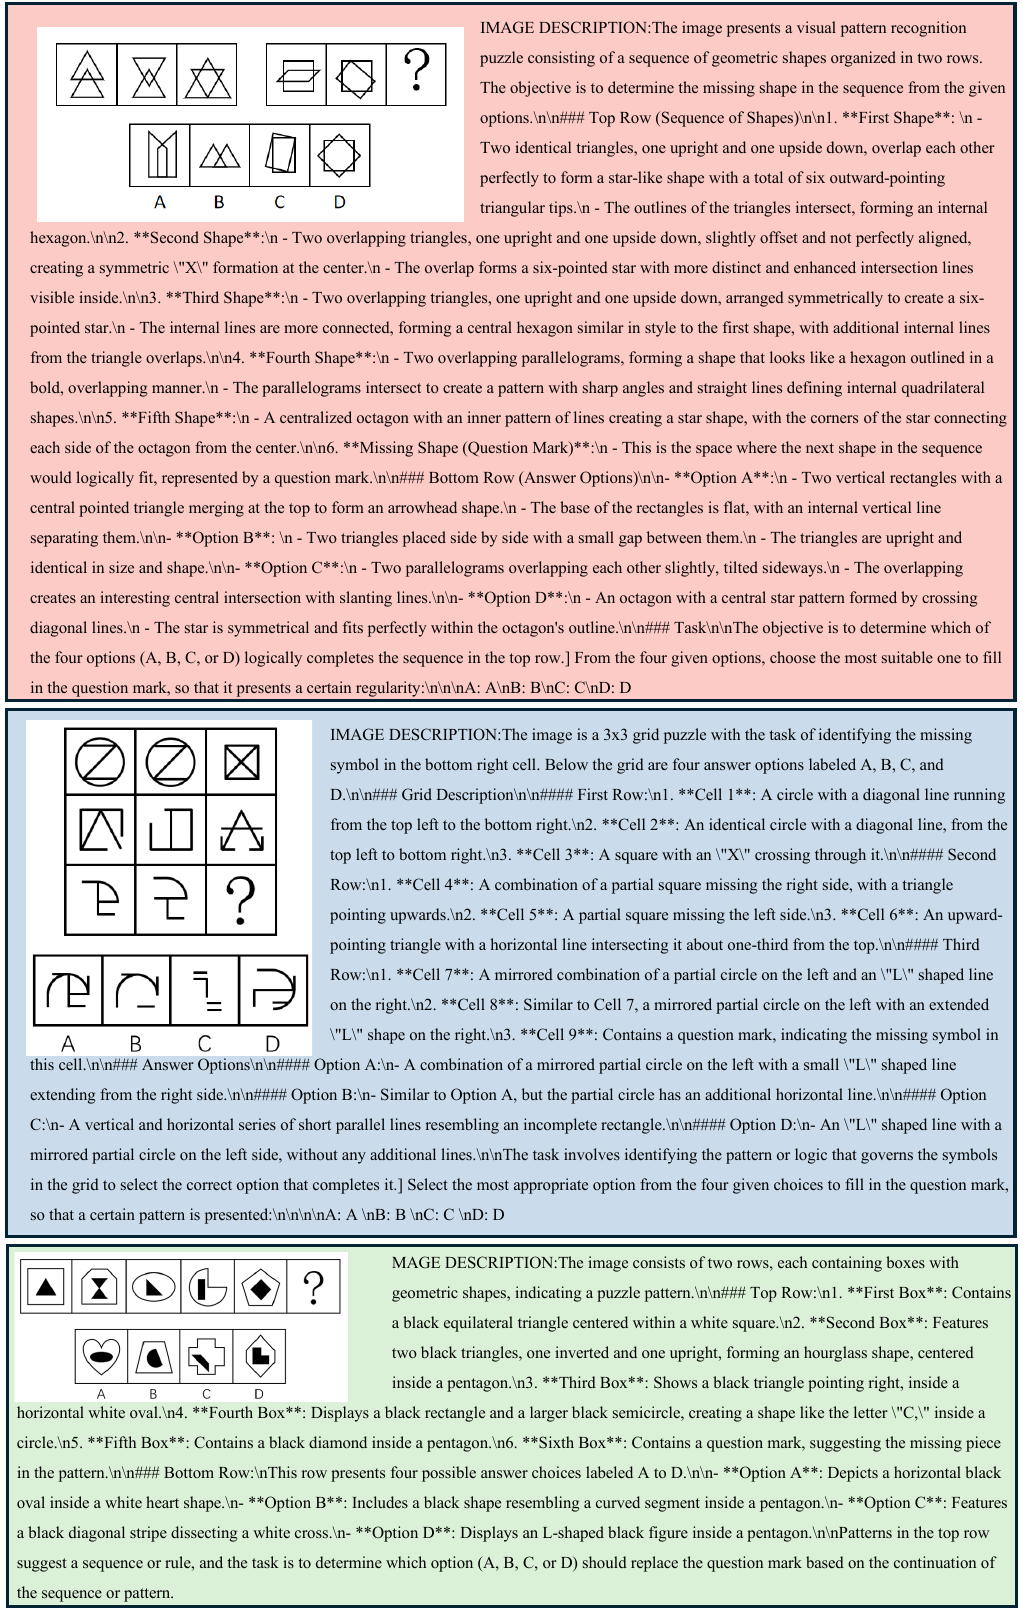}
    \caption{Part of image caption in LLM experiment.}
    \label{fig:image_cation1}
\end{figure}
\begin{figure}
    \centering
    \includegraphics[width=1\linewidth]{images/appendix_image_caption.pdf}
    \caption{Part of image caption in LLM experiment.}
    \label{fig:image_cation2}
\end{figure}
