# Supplementary material for: VisuLogic: A Benchmark for Evaluating Visual Reasoning in Multi-modal Large Language Models
Source: arXiv:2504.15279 source file (2025-04-21)
Supplement: Supplementary file 3 [file model_output.tex]

\section{Model Output Examples}
\begin{figure}
    \centering
    \includegraphics[width=1\linewidth]{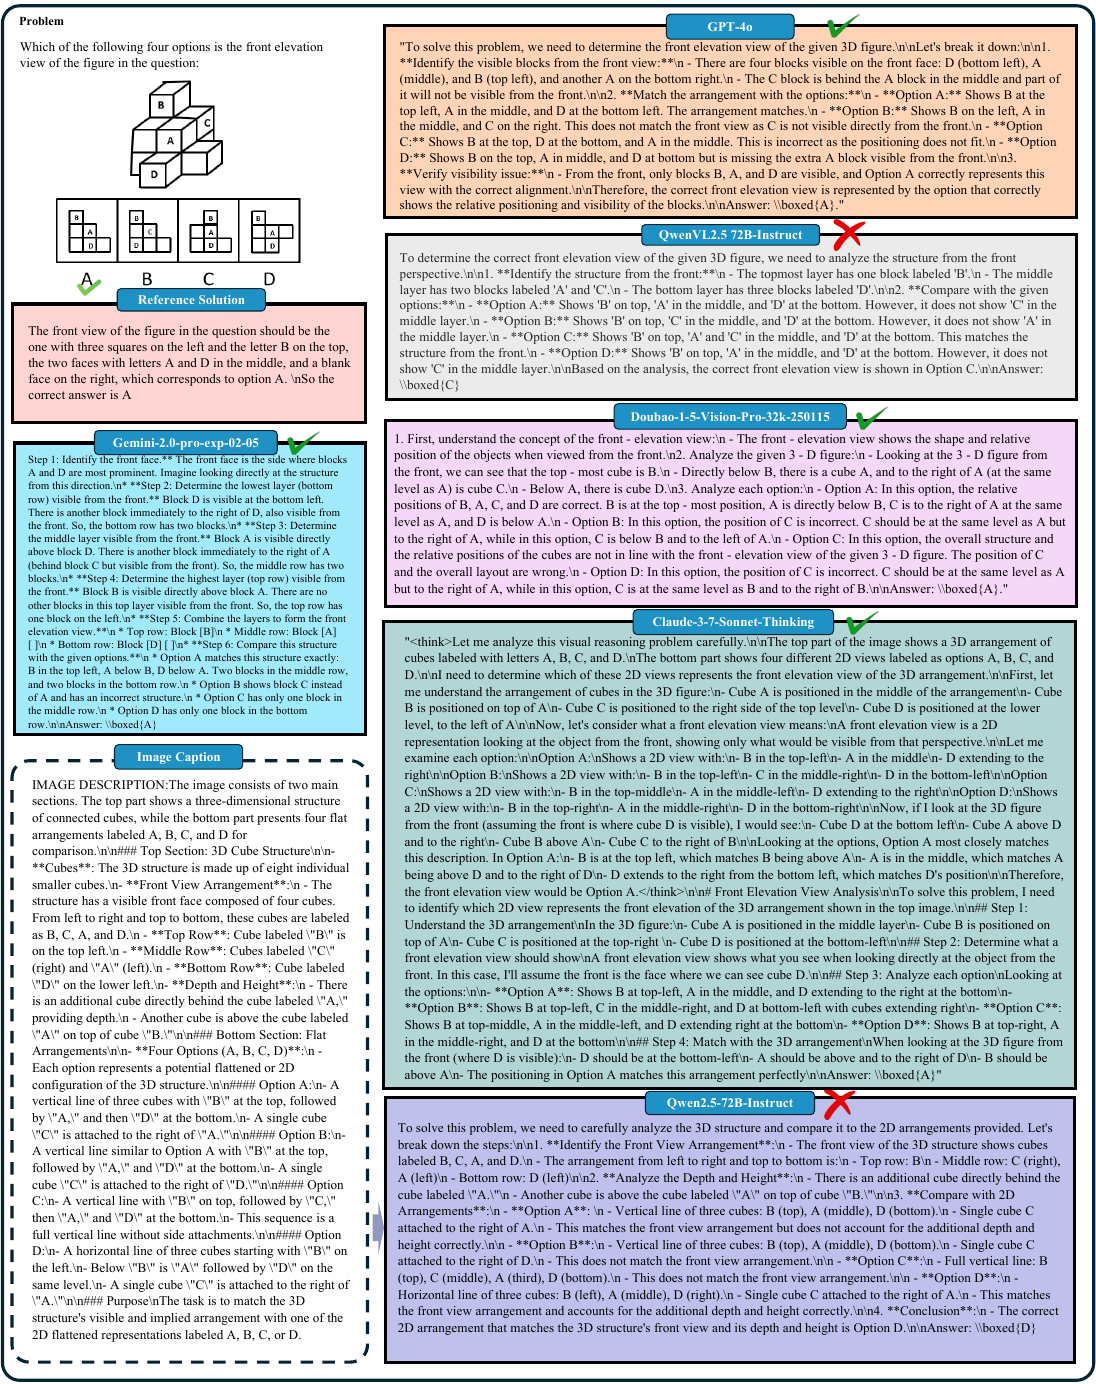}
    \caption{Enter Caption}
    \label{fig:enter-label}
\end{figure}
\begin{figure}
    \centering
    \includegraphics[width=1\linewidth]{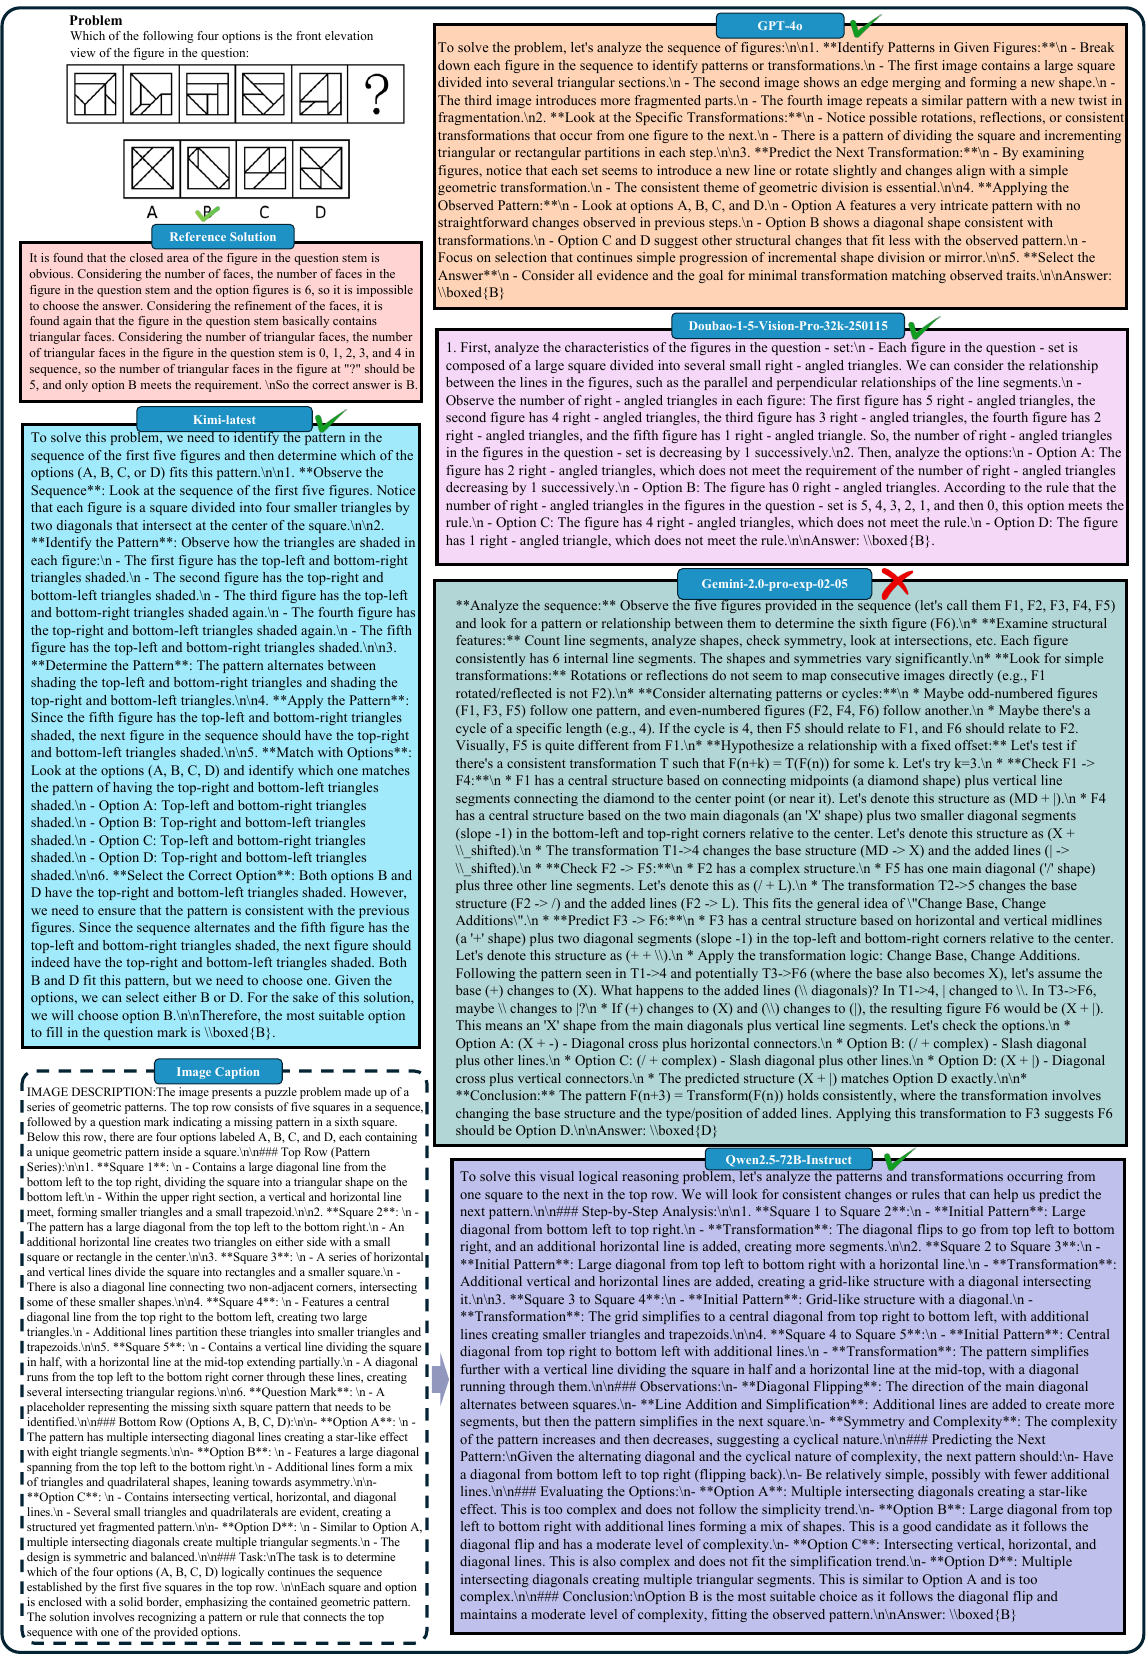}
    \caption{Enter Caption}
    \label{fig:enter-label}
\end{figure}
